# Supplementary material for: A convex relaxation to compute the nearest structured rank deficient matrix
Source: arXiv:1904.09661 source file (2020-10-09)
Supplement: Supplementary file 1 [file additionalproofs.tex]

\section{Additional proofs}\label{s:additionalproofs}

\begin{lemma}\label{thm:idealsequal}
  $\mathcal{J}=\mathcal{J}'$, where
  $\mathcal{J}' := \langle p_i^T x,\; x^TE x - 1,\; x_{l_1}x_{l_2}-x_{l_3}x_{l_4} \rangle.$
\end{lemma}
\begin{proof}
  It is clear that $\mathcal{J}\subset \mathcal{J}'$.
  Let us prove now that $\mathcal{J}'\subset \mathcal{J}$.
  First notice that the rank one equations $x_{l_1}x_{l_2}-x_{l_3}x_{l_4}$ imply that
  $$x^T(p_ie_j^T)x \equiv_\mathcal{J} x^T\sym(p_ie_j^T)x\equiv_\mathcal{J} 0,$$
  and thus $(p_i^Tx)x_j \in \mathcal{J}$.
  Note that the entries of $x$ can be indexed by pairs $(j_1,j_2)$ with $0\leq j_1\leq n$, $1\leq j_2\leq k$.
  Observe that
  \begin{align*}
    p_i^T x \equiv_\mathcal{J} (p_i^Tx)(x^TEx) = \sum_{j_2} (p_i^Tx)x_{(0,j_2)}^2 \equiv_\mathcal{J} 0,
  \end{align*}
  and thus $p_i^T x \in \mathcal{J}$, as wanted.
\end{proof}

\begin{proof}[Proof of \Cref{thm:isomorphism}]
  Consider the map $\phi: \RR[x]/\mathcal{J}' \to \RR[v,z]/\langle{h}\rangle \to $ such that
  $f(x)\mapsto g(v,z):=f(\vone\otimes z)$.
  It is easy to see that $\phi$ is a well-defined homomorphism.
  Moreover, it is an isomorphism, whose inverse map is
  $g(v,z)\mapsto f(x):=g(\bar{v}(x),\bar{z}(x))$
  where
  $
    \bar{z}_{j}(x) := x_{(0,j)}$  and $ \bar{v}_i(x) := \sum_{j} x_{(i,j)}x_{(0,j)}.
  $
\end{proof}

\begin{proof}[Proof of \Cref{thm:quadraticforms}]
  Let $\RR[t]_d$ be the space of forms of degree~$d$ in $k$ variables.
  Observe that $\RR^k, \SS^k$ are in correspondence with $\RR[t]_1,\RR[t]_2$.
  The first item follows by noticing that if some linear forms $\{\ell_i(t)\}_i$ span $\RR[t]_1$ then $\{t_j \ell_i(t)\}_{ij}$ span $\RR[t]_2$.
  For the second item, it is clear that $\zeta\zeta^T \in L_2^\perp$, so it suffices to see that $\{\zeta\zeta^T\} \cup L_2 $ span $\SS^k$.
  This corresponds to the simple fact that if $\{\hat{\ell}\}\cup \{\ell_i(t)\}_i$ span $\RR[t]_1$ then $\{\hat{\ell}^2\}\cup \{t_j \ell_i(t)\}_{ij}$ span $\RR[t]_2$.
\end{proof}
